# Supplementary material for: OmniMVS: End-to-End Learning for Omnidirectional Stereo Matching
Source: arXiv:1908.06257 source file (2019-08-17)
Supplement: Supplementary file 1 [file iccv-supp.pdf]

# OmniMVS: End-to-End Learning for Omnidirectional Stereo Matching

Changhee Won, Jongbin Ryu and Jongwoo Lim\*

Department of Computer Science, Hanyang University, Seoul, Korea.

{chwon, jongbinryu, jlim}@hanyang.ac.kr

## Supplementary Material

### 1. Details of Proposed Datasets

**OmniThings** The proposed OmniThings dataset is built for training and testing large scale stereo correspondences in various photometric and geometric environments. 64 shapes are randomly selected from ShapeNet [1], and they are applied by random textures and similarity transformations. We elaborately place the objects in the virtual scenes following [4]. To place the  $i$ -th object, its position in the rig coordinate system is determined as

$$\mathbf{P}_i = d_i(2u_i\sqrt{1-s_i}, 2v_i\sqrt{1-s_i}, 1-2s_i)^\top,$$

where  $u_i$  and  $v_i$  are randomly sampled with the constraint  $s_i = u_i^2 + v_i^2 < 1$ , and  $d_i$  represents a random distance.

Collision check of the newly placed object is performed by testing the overlap of the bounding boxes of the objects. For 70% scenes, we generate cuboid rooms with random aspect ratios, textures, and transformations, and for the rest, skies with different weathers at infinite distance for learning the background model.

**OmniHouse** We also propose Omnihouse dataset for learning various indoor environments. Synthesized indoor scenes are reproduced using the models in SUNCG dataset [5] and a few additional models. We collect 451 house models consisting of various rooms and objects (*e.g.*, beds and sofas) with the sunny sky background. To generate more data, multiple images are rendered for each 3D scene at random positions and orientations.

Figure 1 shows the effectiveness of using our datasets. The results named ‘OmniMVS’ are by the model trained on OmniThings dataset only, and ‘OmniMVS-ft’ is by the model fine-tuned on Sunny [6] and OmniHouse datasets. Both networks perform well on the textured regions whereas OmniMVS-ft performs favorably to OmniMVS on the textureless or reflective surfaces. Additional examples of our proposed datasets are also shown in Fig. 2 and 3.

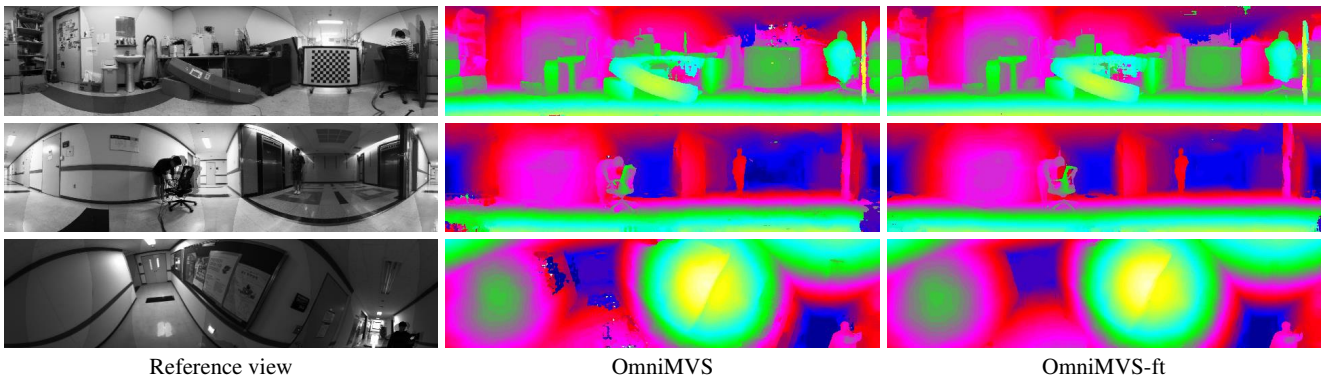

Figure 1: **Effectiveness of our datasets on the real data.** OmniMVS is trained using OmniThings. Then, OmniMVS-ft is fine-tuned on Sunny [6] and OmniHouse.

| Dataset Metric |                 | OmniThings   |              |              |             |             | OmniHouse    |              |             |             |             |
|----------------|-----------------|--------------|--------------|--------------|-------------|-------------|--------------|--------------|-------------|-------------|-------------|
|                |                 | >1           | >3           | >5           | MAE         | RMS         | >1           | >3           | >5          | MAE         | RMS         |
| RGB            | PSMNet [2]      | 86.25        | 63.23        | 44.84        | 7.28        | 11.15       | 63.22        | 26.43        | 15.39       | 5.82        | 13.88       |
|                | PSMNet-ft       | 82.69        | 51.98        | 41.74        | 9.09        | 13.71       | 87.56        | 27.01        | 12.89       | 3.51        | 6.05        |
|                | DispNet-CSS [3] | <b>50.62</b> | <b>27.77</b> | <b>19.50</b> | <b>4.06</b> | <b>7.98</b> | <b>26.56</b> | <b>11.69</b> | <b>7.16</b> | <b>1.54</b> | <b>3.18</b> |
|                | DispNet-CSS-ft  | 67.86        | 48.08        | 38.57        | 7.81        | 12.27       | 36.47        | 14.98        | 8.29        | 1.81        | 3.44        |
| Gray           | PSMNet          | 86.77        | 64.33        | 45.78        | 7.42        | 10.72       | 64.32        | 25.48        | 13.59       | 4.40        | 10.61       |
|                | PSMNet-ft       | 82.64        | 51.70        | 41.69        | 9.16        | 13.83       | 87.70        | 26.90        | 13.12       | 3.56        | 6.18        |
|                | DispNet-CSS     | 50.64        | 27.92        | 19.62        | 4.06        | 8.00        | 26.61        | 11.83        | 7.30        | 1.56        | 3.22        |
|                | DispNet-CSS-ft  | 67.90        | 48.24        | 38.76        | 7.89        | 12.37       | 36.48        | 15.08        | 8.46        | 1.82        | 3.46        |

  

| Dataset Metric |                | Sunny        |             |             |             |             | Cloudy       |             |             |             |             | Sunset       |             |             |             |             |
|----------------|----------------|--------------|-------------|-------------|-------------|-------------|--------------|-------------|-------------|-------------|-------------|--------------|-------------|-------------|-------------|-------------|
|                |                | >1           | >3          | >5          | MAE         | RMS         | >1           | >3          | >5          | MAE         | RMS         | >1           | >3          | >5          | MAE         | RMS         |
| RGB            | PSMNet         | 65.09        | 30.87       | 13.13       | 2.54        | 4.03        | 63.62        | 28.51       | 10.40       | 2.45        | 4.26        | 63.83        | 28.41       | 10.00       | 2.43        | 4.11        |
|                | PSMNet-ft      | 92.67        | 31.45       | 21.32       | 4.33        | 7.76        | 92.92        | 31.24       | 20.14       | 4.13        | 7.32        | 93.24        | 30.64       | 19.65       | 4.11        | 7.43        |
|                | DispNet-CSS    | <b>24.80</b> | 8.54        | 5.59        | 1.44        | 4.02        | 25.16        | <b>8.47</b> | <b>5.50</b> | <b>1.43</b> | <b>3.92</b> | 24.79        | <b>8.29</b> | <b>5.34</b> | <b>1.38</b> | <b>3.76</b> |
|                | DispNet-CSS-ft | 39.02        | 21.12       | 14.47       | 2.37        | 4.85        | 42.29        | 21.55       | 14.28       | 2.43        | 4.88        | 40.21        | 20.91       | 14.43       | 2.40        | 4.88        |
| Gray           | PSMNet         | 61.57        | 28.19       | 10.15       | 2.40        | 4.18        | 65.08        | 30.64       | 12.64       | 2.52        | 4.05        | 65.39        | 30.59       | 12.74       | 2.52        | 4.00        |
|                | PSMNet-ft      | 93.10        | 31.08       | 20.02       | 4.10        | 7.20        | 92.90        | 31.14       | 20.76       | 4.16        | 7.36        | 92.94        | 31.01       | 20.94       | 4.20        | 7.61        |
|                | DispNet-CSS    | 25.09        | <b>8.51</b> | <b>5.54</b> | <b>1.43</b> | <b>3.98</b> | <b>25.06</b> | 8.62        | 5.67        | 1.46        | 4.01        | <b>24.69</b> | 8.55        | 5.55        | 1.41        | 3.88        |
|                | DispNet-CSS-ft | 38.83        | 20.71       | 13.81       | 2.33        | 4.77        | 42.93        | 21.76       | 14.50       | 2.45        | 4.90        | 39.93        | 21.07       | 14.54       | 2.40        | 4.87        |

Table 1: **Quantitative comparison between using RGB and grayscale input image for stitching conventional stereo.** The qualifier '>n' refers to the pixel ratio (%) whose error is larger than n, 'MAE' refers to the mean absolute error, and 'RMS' refers to the root mean squared error. The errors are averaged over all test frames of each datasets.

## 2. Grayscale Input for Conventional Stereo

Although many conventional stereo methods, PSMNet [2] and DispNet-CSS [3], are trained on the RGB input images, our proposed networks use the grayscale images. In this section we verify the performance differences between using RGB and grayscale images for the conventional methods. We replicate grayscale images to the 3 channel to match the network architecture. As shown in Table 1, the results with grayscale input are almost the same or slightly lower than those with RGB input.

## 3. Supplementary Video

We present the overview of the proposed OmniMVS and our datasets, and additional experiments on the real data. Please see the video at <https://www.youtube.com/watch?v=6DKen2MQocQ>.

## References

- [1] Angel X Chang, Thomas Funkhouser, Leonidas Guibas, Pat Hanrahan, Qixing Huang, Zimo Li, Silvio Savarese, Manolis Savva, Shuran Song, Hao Su, et al. Shapenet: An information-rich 3d model repository. *arXiv preprint arXiv:1512.03012*, 2015. 1
- [2] Jia-Ren Chang and Yong-Sheng Chen. Pyramid stereo matching network. In *Proceedings of the IEEE Conference on Computer Vision and Pattern Recognition*, pages 5410–5418, 2018. 2
- [3] Eddy Ilg, Tonmoy Saikia, Margret Keuper, and Thomas Brox. Occlusions, motion and depth boundaries with a generic network for disparity, optical flow or scene flow estimation. In *Proceedings of the European Conference on Computer Vision (ECCV)*, pages 614–630, 2018. 2
- [4] George Marsaglia et al. Choosing a point from the surface of a sphere. *The Annals of Mathematical Statistics*, 43(2):645–646, 1972. 1
- [5] Shuran Song, Fisher Yu, Andy Zeng, Angel X Chang, Manolis Savva, and Thomas Funkhouser. Semantic scene completion from a single depth image. *IEEE Conference on Computer Vision and Pattern Recognition*, 2017. 1
- [6] Changhee Won, Jongbin Ryu, and Jongwoo Lim. Sweepnet: Wide-baseline omnidirectional depth estimation. *arXiv preprint arXiv:1902.10904*, 2019. 1

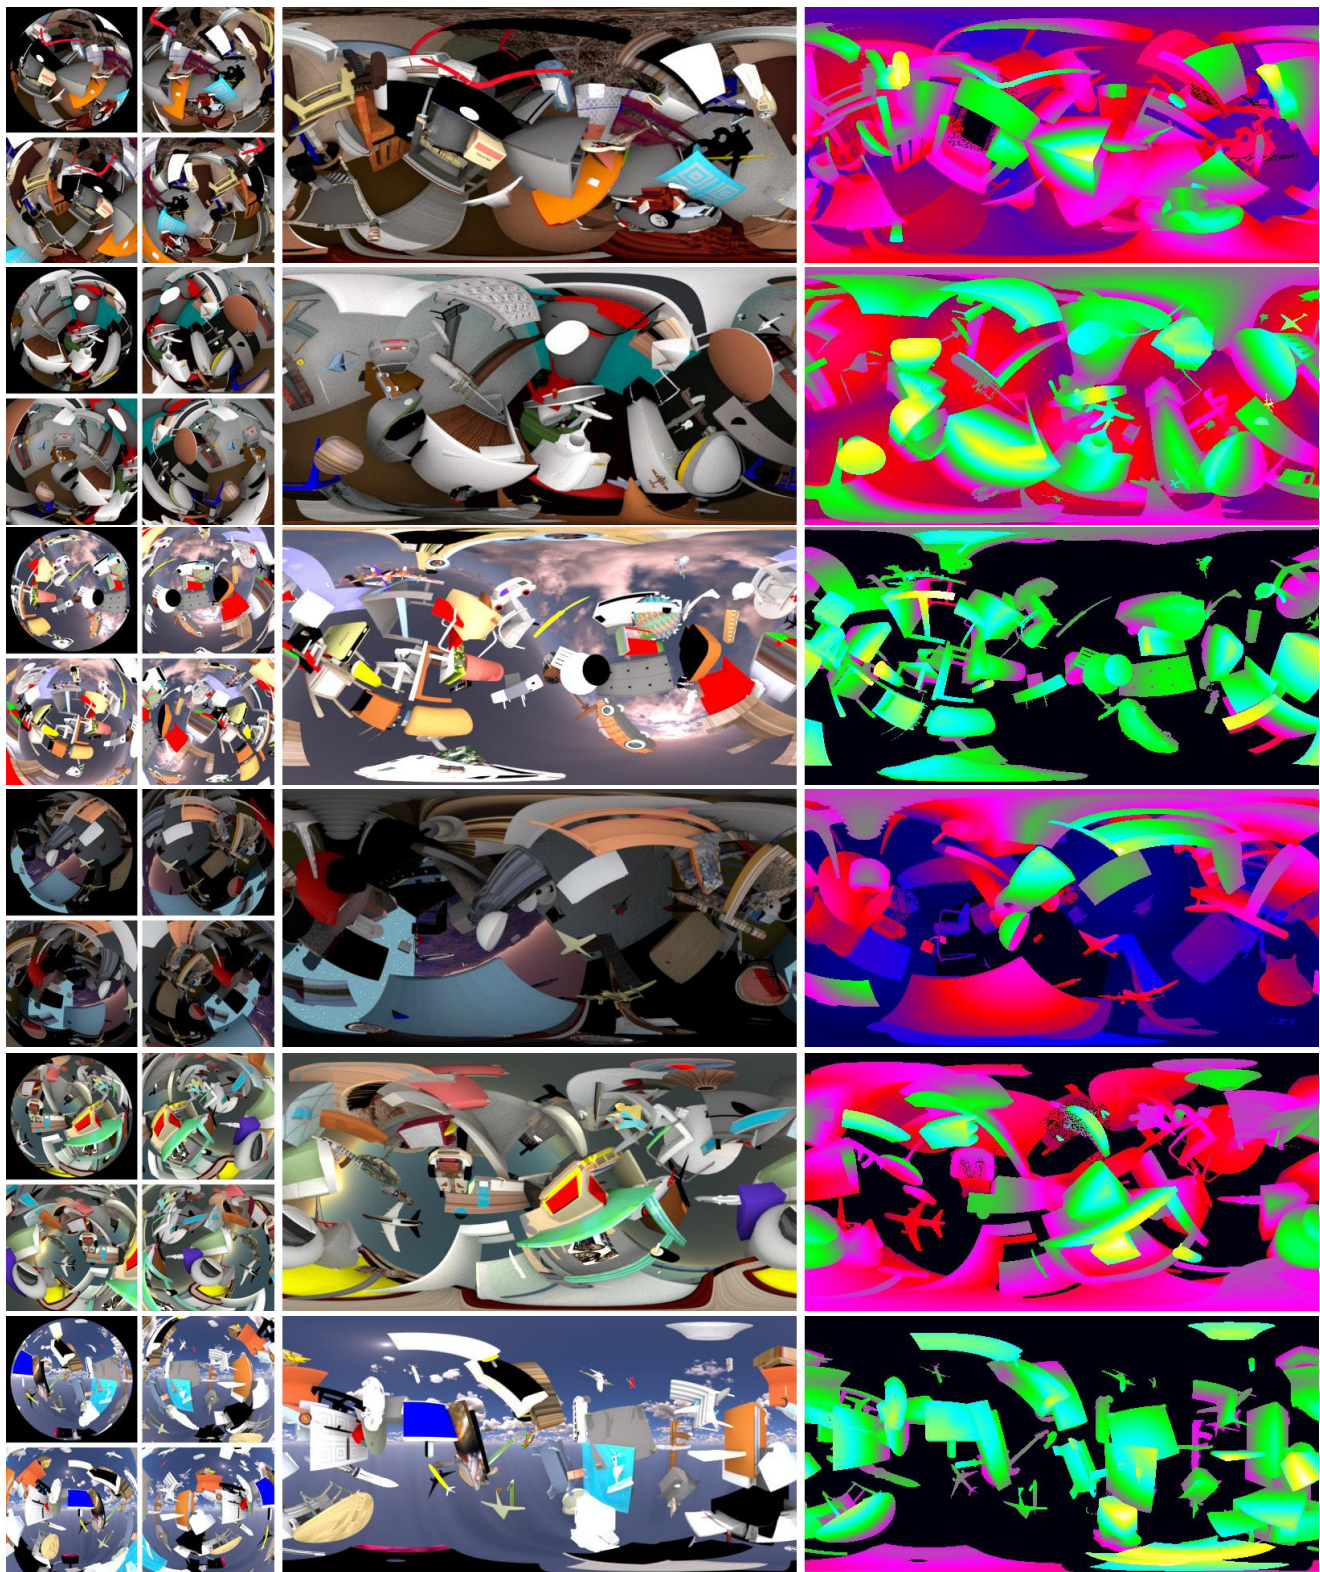

Figure 2: **OmniThings**. From left: input fisheye images, reference panorama image, and ground truth inverse depth map.

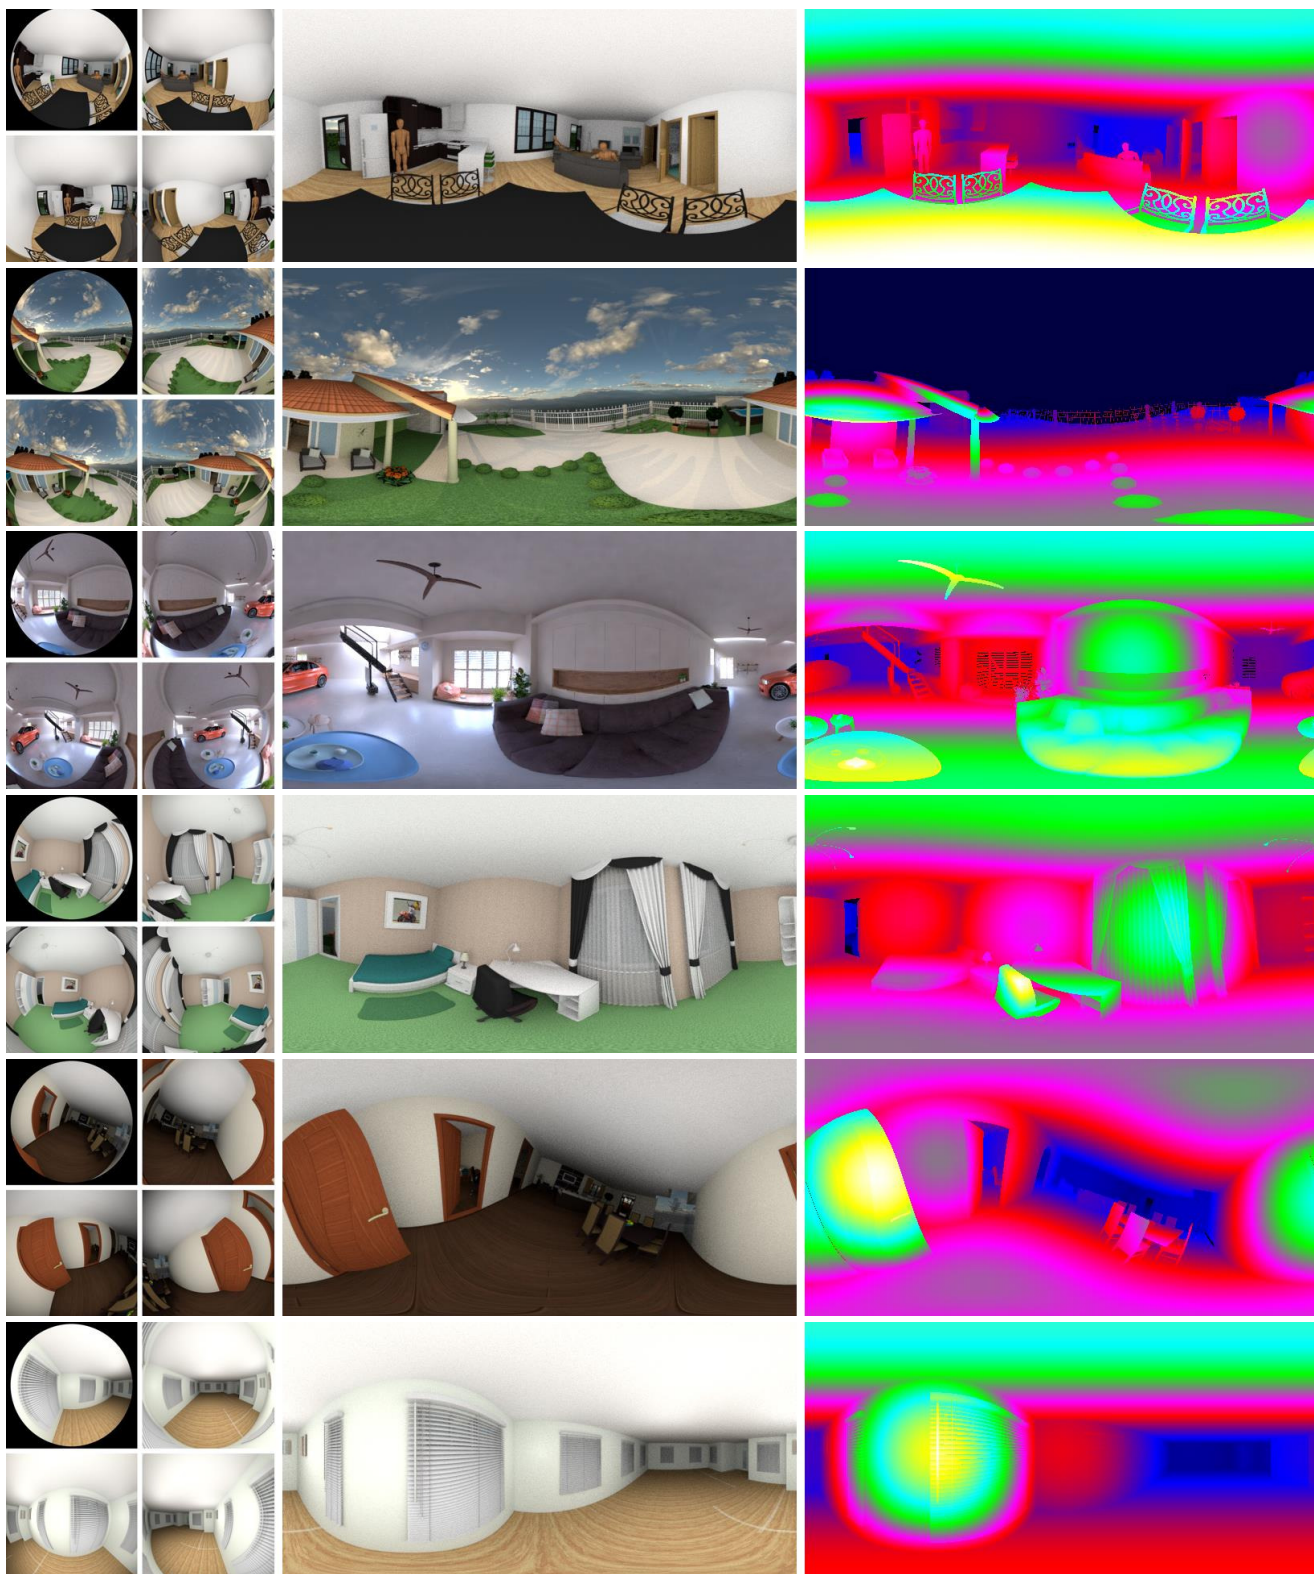

Figure 3: **OmniHouse**. From left: input fisheye images, reference panorama image, and ground truth inverse depth map.
